# Supplementary material for: Effects of infection fatality ratio and social contact matrices on vaccine prioritization strategies
Source: arXiv:2201.02869 ancillary file (2022-08-07)
Supplement: Supplementary file 1 [file covid19-vac_supp.pdf]

# Supplemental Information for "Effects of infection fatality ratio and social contact matrices on vaccine prioritization strategies"

Arthur Schulenburg [1], Wesley Cota [1], Guilherme S. Costa [1], and Silvio C. Ferreira [1,2]

[1] Departamento de Fisica, Universidade Federal de Viçosa, 36570-900 Viçosa, Minas Gerais, Brazil
[2] National Institute of Science and Technology for Complex Systems, 22290-180 Rio de Janeiro, Brazil

(Dated: June 26, 2022)

## CONTENTS

SI-I. Demography and contact structure of Uganda and Germany 1

SI-II. Impact of DAP vaccination for an ideal vaccine model 3

SI-III. Reduction of recovered individuals with age-dependent values of efficiency 4

SI-IV. Optimal and least effective strategies using Uganda and Germany contact patterns 5

SI-V. Optimal and least effective strategies for young, adults and elderly populations 6

References 8

## SI-I. DEMOGRAPHY AND CONTACT STRUCTURE OF UGANDA AND GERMANY

Figures SI-1 and SI-2 present the demographic and contact information for Uganda and Germany, respectively. The respective result for Brazil is available in Fig. 2 of the main paper.

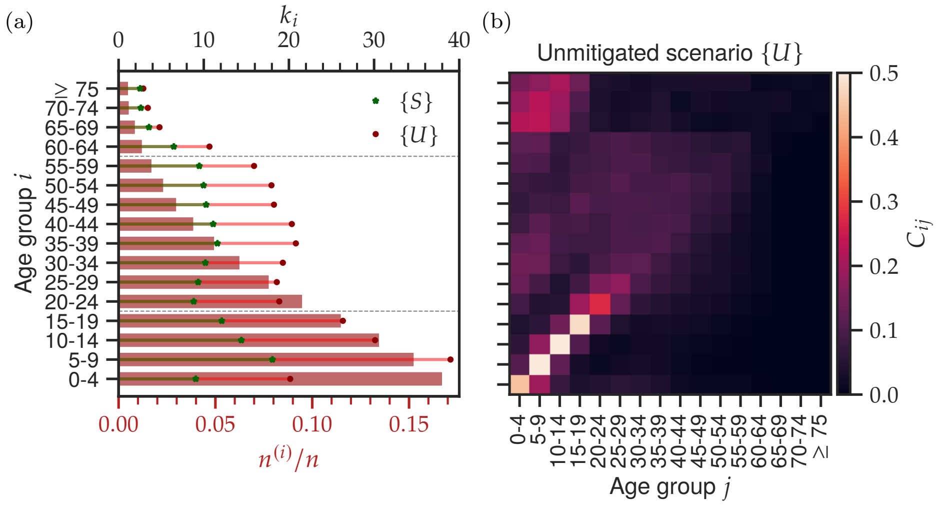


FIG. SI-1. Demographic and contact patterns in Uganda. (a) Fraction of individuals $n^{(i)}/n$ for each age group $i$ (bars) and their mean number of contacts $k_i$ (symbols) for social distancing and unmitigated scenarios. Lines represent the increase from one scenario to the other. (b) Contact matrix $C_{ij}$ in the unmitigated scenario of Uganda. Data adapted from Refs. [1, 2] as described in the main text.

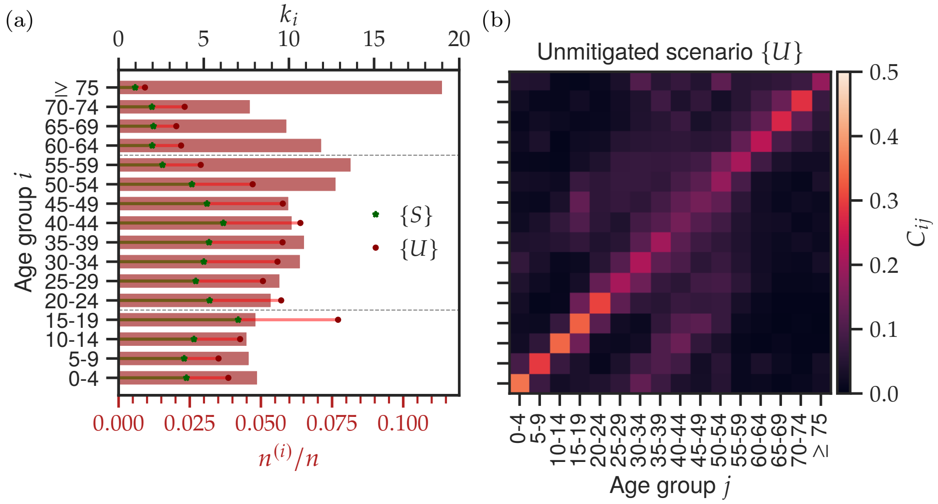


FIG. SI-2. Demographic and contact patterns in Germany. (a) Fraction of individuals $n^{(i)}/n$ for each age group $i$ (bars) and their mean number of contacts $k_i$ (symbols) for social distancing and unmitigated scenarios. Lines represent the increase from one scenario to the other. (b) Contact matrix $C_{ij}$ in the unmitigated scenario of Germany. Data adapted from Refs. [1, 2] as described in the main text.

## SI-II. IMPACT OF DAP VACCINATION FOR AN IDEAL VACCINE MODEL

Figure. SI-3 is equivalent to Fig. 6 of the main paper replacing the realistic model for vaccine efficacy by the profile with uniform values of the ideal model; see Fig. 5 of the main paper.

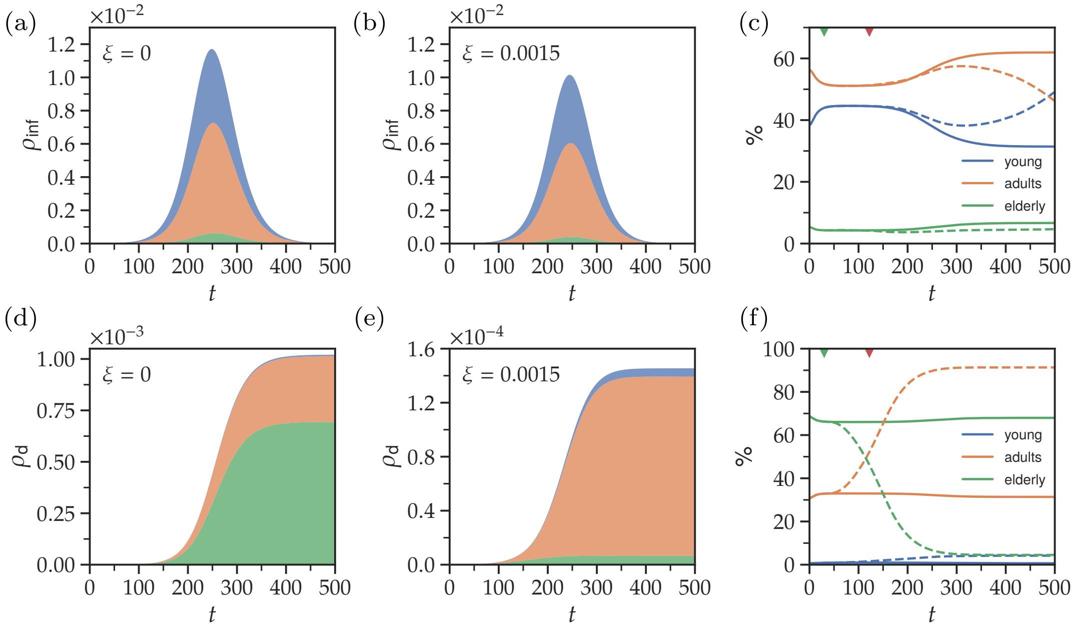


FIG. SI-3. Evolution of the fraction and age profiles of (a-c) infectious individuals and (d-e) accumulated deaths. The effects of DAP strategy with uniform values of efficacy against infection and death are addressed with fixed vaccination rate $\xi = 0.15\%$ and delay of $t_v = 30$ days in a scenario of social distancing with $\omega = R_0^{\{S\}} = 1.3$. In the stack plots, the envelope gives total prevalence or deaths while the colors the proportion within the young (0–19 yr, blue), adult (20–59 yr, orange), and elderly ($\geq 60$ yr, green) age groups. The age profiles for (c) infectious and (f) accumulated deaths give the percentage distribution for each group with (dashed lines) and without (solid lines) vaccination. Triangles indicate when the vaccinations of the elderly and adult population start while in the young population it has not started in the investigated time window. Note that the scales in (d) and (e) are different.

## SI-III. REDUCTION OF RECOVERED INDIVIDUALS WITH AGE-DEPENDENT VALUES OF EFFICIENCY

Figure SI-4 present the reduction in the number of recovered individuals (R, $R_V$, and $R_P$), adopting the DAP strategy with Brazil's demographics and contact matrices and the same parameters of Fig. 7 in the main paper. Note that the reduction is negligible for the unmitigated scenario.

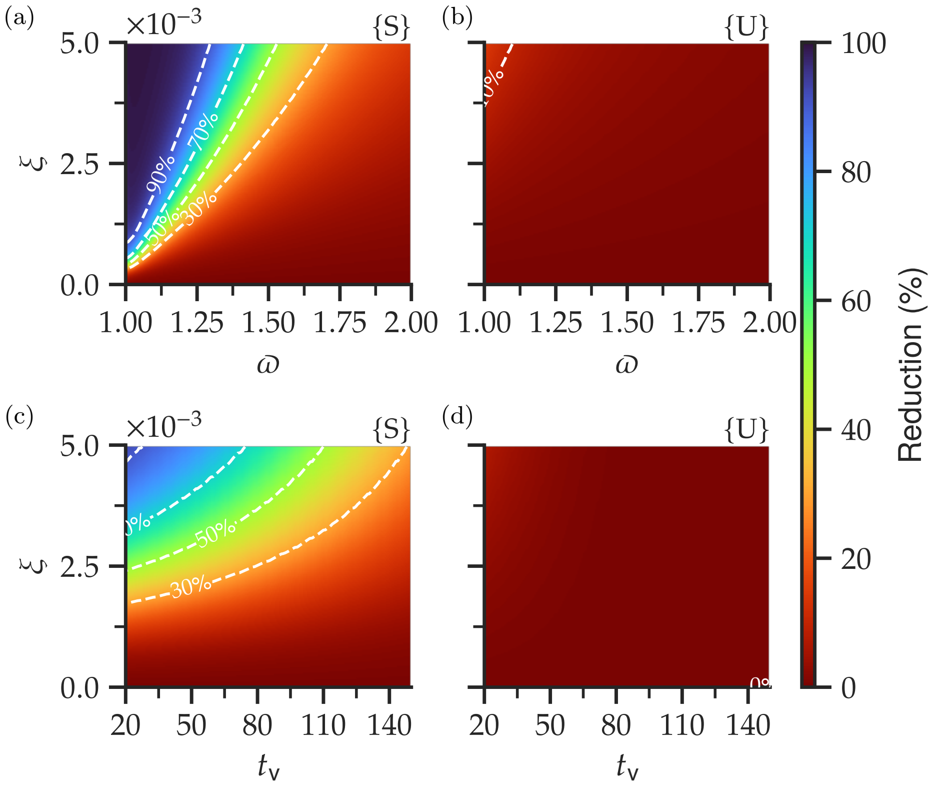


FIG. SI-4. Heatmaps and isolines (white curves) for reduction of recovered individuals using a DAP strategy and age-dependent values of efficacy against death and infection (realistic model of Fig. 5 of the main paper) in comparison to the situation without vaccines in space parameters (a,b) $\xi \times \varpi$ for $t_v = 30$ days and (c,d) $\xi \times t_v$ for $\omega = 1.3$. (a,c) Social distancing and (b,d) unmitigated scenarios are presented.

## SI-IV. OPTIMAL AND LEAST EFFECTIVE STRATEGIES USING UGANDA AND GERMANY CONTACT PATTERNS

In Fig. SI-5 we show the optimal and least effective strategies for the contact and demographic patterns of Uganda and Germany with COVID-19's IFR age-profile, uniform efficiency against deaths and infections, and the remaining epidemic parameters are the same as Fig. 8 in the main paper.

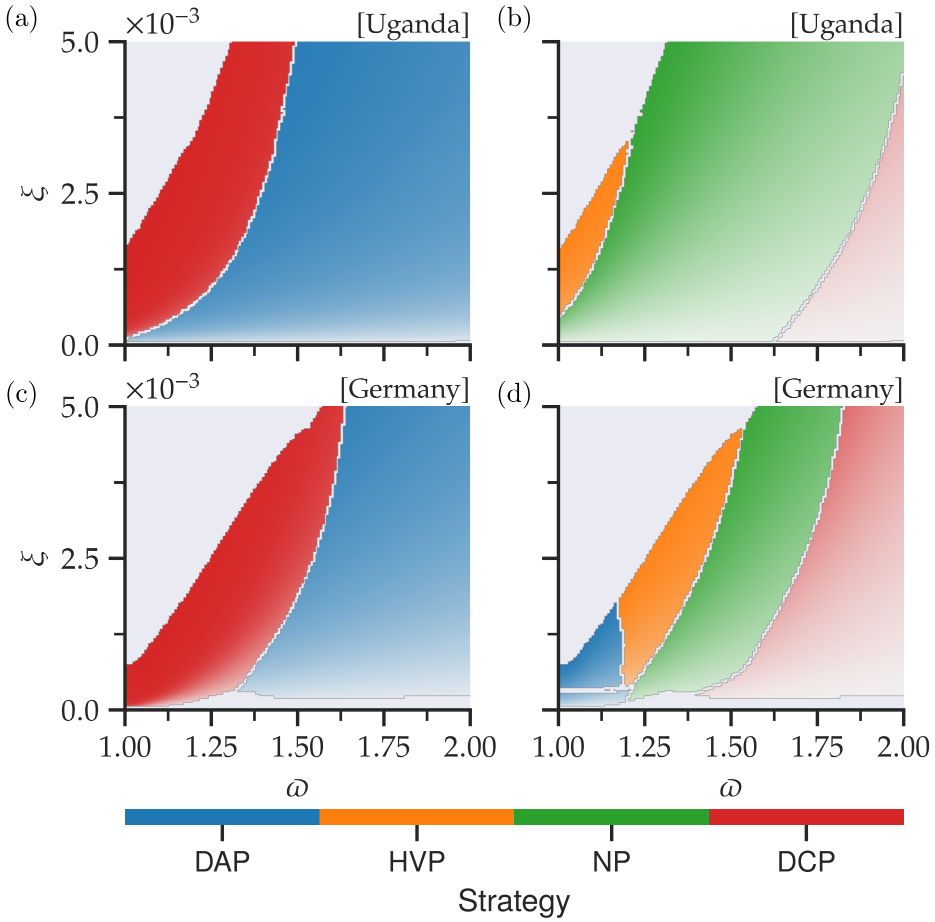


FIG. SI-5. Diagrams indicating the most (left) and least (right) effective strategies for reduction of deaths in the total population in the space parameter $\omega$ versus $\xi$ using the COVID-19's IFR for Uganda (top) and Germany (bottom). Four vaccination strategies defined in the main text are considered: decreasing age (DAP), highly vulnerable (HVP), no (NP), and decreasing contact (DCP) prioritizations. A time delay of $t_v = 30$ days, vaccination with uniform values of efficacy against death and infection, and social distancing contact scenario were considered. The gradient colors refer to the respective reduction of deaths, the darker the highest. Differences between the most and least effective strategies smaller than 5% are depicted in gray.

## SI-V. OPTIMAL AND LEAST EFFECTIVE STRATEGIES FOR YOUNG, ADULTS AND ELDERLY POPULATIONS

In Figs. SI-6 and SI-7 we perform the analysis done in Fig. 10 of the main paper focusing on the optimal and least effective strategies, respectively, for each age-group of young, adults, and elderly individuals considering a social distancing scenario and COVID-19's IFR age-profile. Prioritization of higher contact is most effective to reduce deaths in the young population while age prioritization is least effective to prevent deaths in this group. Notice, however, that the total number of deaths is highly concentrated in the elderly population and the diagrams for the whole population resemble very much those for the elderly.

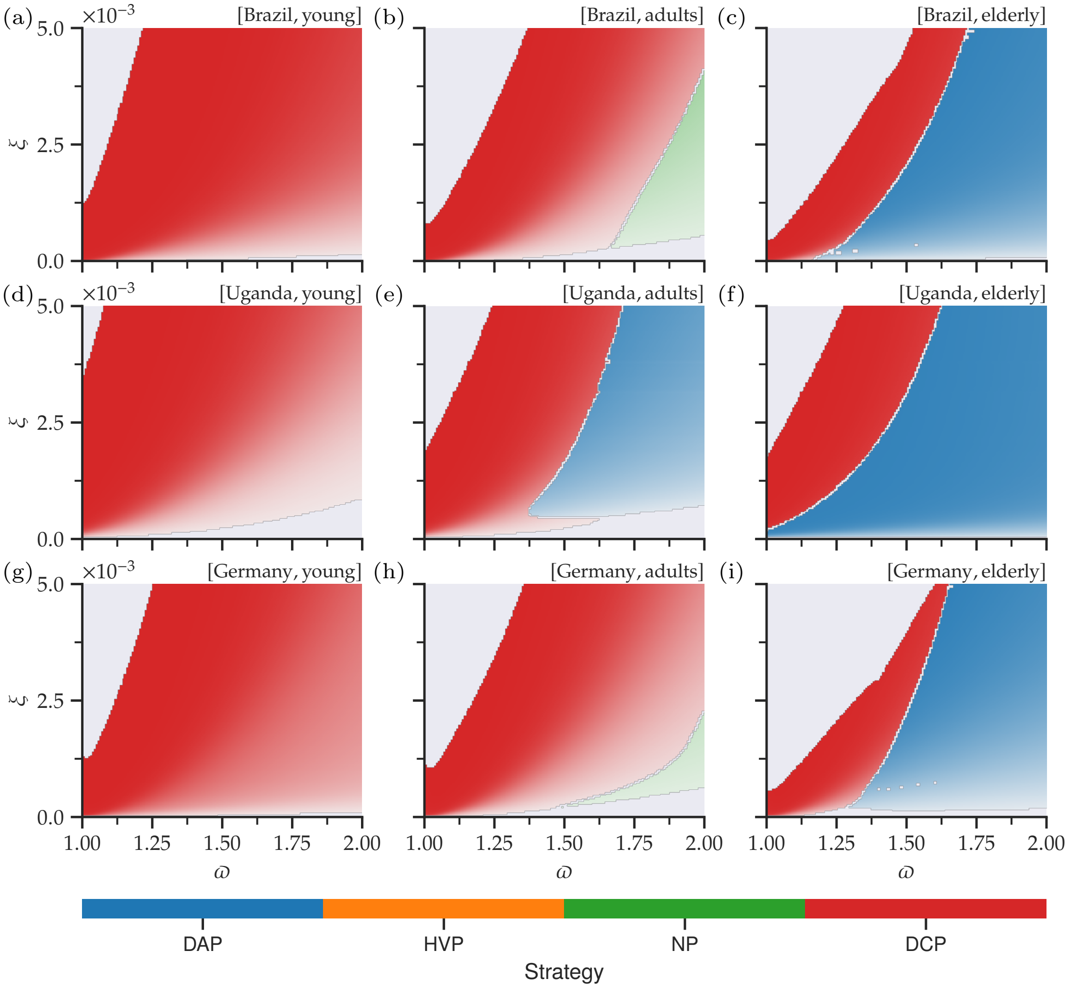


FIG. SI-6. Diagrams indicating the optimal strategies in the parameter space $\xi$ versus $\omega$ for (a,d,g) young, (b,e,h) adult, and (c,f,i) elderly populations in (a-c) Brazil, (d-f) Uganda, and (g-i) Germany. The IFR age profile of COVID-19, a time delay of $t_v = 30$ days, vaccination with age-dependent values of efficacy against deaths and infections, and social distancing contact scenario were adopted.

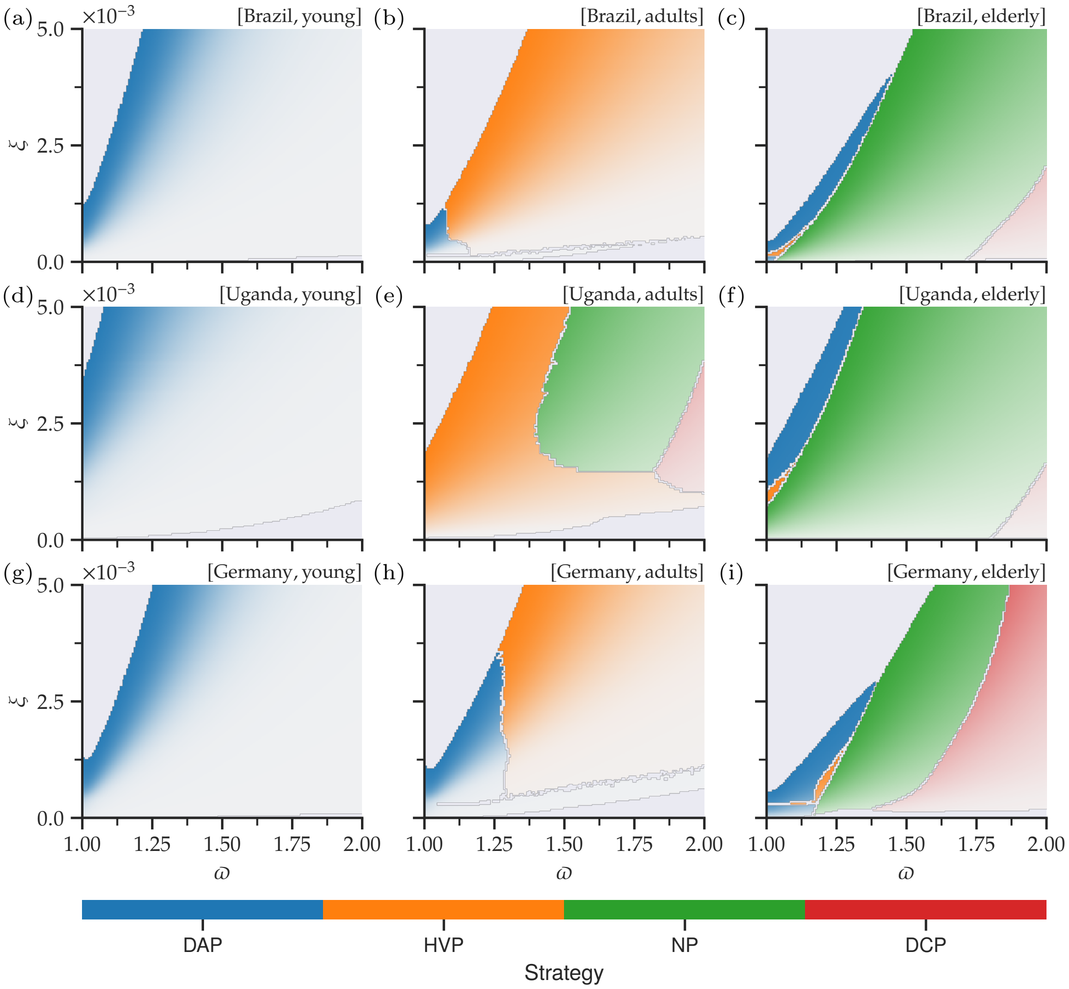


FIG. SI-7. Diagrams indicating the least effective strategies in the parameter space $\xi$ versus $\omega$ for (a,d,g) young, (b,e,h) adult, and (c,f,i) elderly populations in (a-c) Brazil, (d-f) Uganda, and (g-i) Germany. The IFR age profile of COVID-19, a time delay of $t_v = 30$ days, vaccination with age-dependent values of efficacy against death and infection, and social distancing contact scenario were adopted.

[1] United Nations, World Population Prospects 2019, Department of Economic and Social Affairs, Population Division (2019).
[2] K. Prem, A. R. Cook, and M. Jit, Projecting social contact matrices in 152 countries using contact surveys and demographic data, PLOS Comput. Biol. **13**, e1005697 (2017).
